# Supplementary material for: Learned Image Compression with Dictionary-based Entropy Model
Source: arXiv:2504.00496 source file (2025-05-15)
Supplement: Supplementary file 1 [file _supplementary.tex]

% \input{_constants}
% % \review % \review OR \cameraready
% \cameraready
% \documentclass[10pt,onecolumn,letterpaper]{article}
% \input{cvpr_header}
% \myexternaldocument{_main}
% \begin{document}

% %% TITLE
% \title{\paperTitle}
% \author{\authorBlock}
% \maketitlesupplementary
% %%
% \appendix
% \input{12_appendix}

% \end{document}
